# Supplementary material for: Noiseless quantum measurement and squeezing of microwave fields utilizing mechanical vibrations
Source: arXiv:1610.09980 ancillary file (2016-10-31)
Supplement: Supplementary file 1 [file 2016-10-01-SqueezeAmpSuppl.pdf]

# Noiseless quantum measurement and squeezing of microwave fields utilizing mechanical vibrations: Supplementary Information

C. Ockeloen-Korppi,[1] E. Damskägg,[1] J.-M. Pirkkalainen,[1] T. T. Heikkilä,[2] F. Massel,[2] and M. A. Sillanpää[1]

[1] *Department of Applied Physics, Aalto University, P.O. Box 15100, FI-00076 AALTO, Finland*
[2] *Department of Physics and Nanoscience Center, University of Jyväskylä, P.O. Box 35 (YFL), FI-40014 University of Jyväskylä, Finland*

## I. EXPERIMENTAL DETAILS AND CALIBRATIONS

### A. Bath temperatures and optical spring

The mechanics is coupled to a bath corresponding to the phonon number $n_m^T$. When the mechanical resonator is thermalized to the cryostat temperature $T$, the temperature of the bath simply follows $\hbar\omega_m n_m^T = k_B T$ when $n_m^T \gg 1$. A single pump tone applied at the red sideband will transduce the mode temperature in the motional sideband peaks representing the thermal motion of the mechanics. We observe the regular motional sidebands as shown in Fig. S1a. With a weak pump tone, the bath temperature is expected to appear in the area in the motional sideband peaks, following a linear temperature dependence. The linear behavior is observed down to $\sim 30$ mK (Fig. S1b), below which the local bath, to which the mechanics is coupled, starts to saturate. The equilibrium temperature of the bath, holding at the lowest pump powers, is around 20 mK, corresponding to $n_m^T \sim 40$. This is a representative thermalization figure for samples produced by our fabrication process.

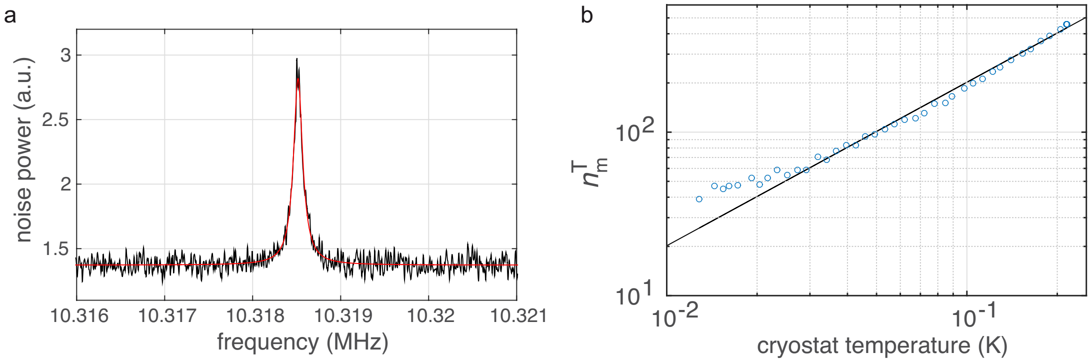


FIG. S1. *Characterizing the mechanical resonator.* **a**, Thermal motion of the mechanics observed in the output spectrum. The solid line is a Lorenzian fit. **b**, Area of the thermal motion peak as a function of cryostat temperature. The solid line is a linear fit using data above $\sim 30$ mK.

However, we usually observe a varying heating of the mechanics bath $n_m^T$ by the pump microwave tone(s), often posing the limiting factor for device performance. We estimate this heating as in main text Ref. [19]. In a previous cooldown on the same sample, we made a rough independent calibration of the bath heating by using sideband cooling. The results are summarized in Fig. S2. We observe an unchanged bath temperature up to $G_- \sim 200$ kHz, followed by a fast increase. In the main text in Fig. 2d and in Fig. S7 (see below), we used as adjustable parameters the values $n_m^T = 80$ and $n_m^T = 220$, respectively, which are somewhat in line with Fig. S2. In Fig. S7, the heating matches with the sideband cooling, but in Fig. 2d, the heating is weaker. We attribute this to our typical observation that the heating varies between cooldowns. A modest heating of the bath representing the cavity internal losses $n_I$ is observed as well.

Under a red-sideband pumping inducing a photon number $n_-$ in the cavity, the radiation-pressure interaction can be linearized, resulting in an effective coupling:

$$G_- = g_0\sqrt{n_-} \gg g_0 \ . \tag{S1}$$

Under these conditions, the optical spring effect enhances the damping of the mechanical resonator by the amount

$$\gamma_{\text{opt}} = \frac{4G_-^2}{\kappa} \ , \tag{S2}$$

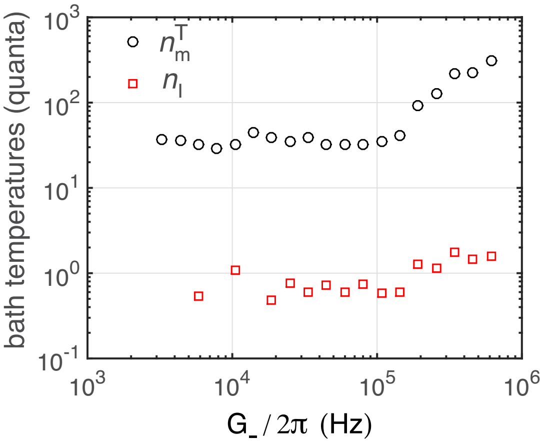


FIG. S2. *Heating of the baths.* Temperatures of the baths of the mechanical resonator (circles), and of the cavity internal bath (squares) as a function of the amplitude of a single pump tone applied to the red sideband, $\omega_- = \omega_c - \omega_m$.

so that the total ("effective") damping of the mechanics is

$$\gamma_{\text{eff}} = \gamma_{\text{opt}} + \gamma \, . \tag{S3}$$

As a consistency check, we verified the expected linear dependence on the added damping (Eq. (S2)) on the generator power, as shown in Fig. S3.

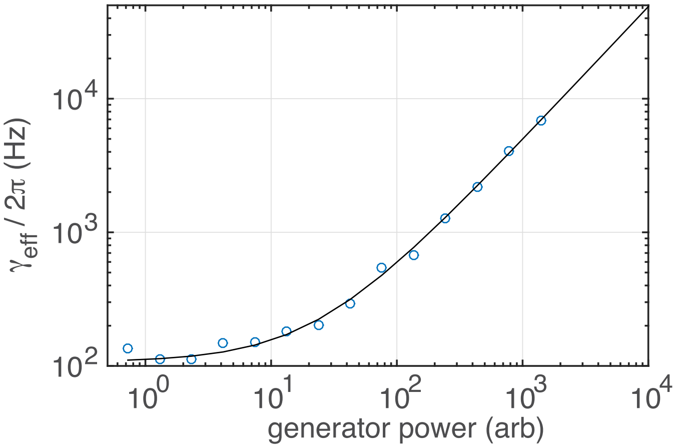


FIG. S3. *Optical spring.* Characterization of the effective linewidth of the mechanical resonator as a function of generator power. The solid line is a linear fit.

### B. Noise calibrations

Let us briefly re-state the noise calibration procedure described in the main text. There is inevitably significant attenuation between the sample and the cryogenic hemt amplifier. The corresponding transmission coefficient is $t < 1$. We denote by $F_0$ the total gain of all the post-amplification including the hemt, and by $N_{F0}$ the corresponding noise temperature.

The noise at the output is

$$P_{\text{RT}} = N_{\text{in}} G t F_0 + N_{\text{add}} G t F_0 + N_{F0} F_0 = N_{\text{in}} G F + \left(N_{\text{add}} + N_F / G\right) G F \tag{S4}$$

where we defined the effective post-amplification gain and noise as $F = t F_0$ and $N_F = N_{F0}/t$.

When Eq. (S4) is plotted with a varying $N_{\text{in}}$, we obtain a straight line with a slope $GF$, and a horizontal axis intercept $N_{\text{in},0}$ satisfying

$$N_{\text{in},0} = N_{\text{add}} + \frac{N_F}{G} \tag{S5}$$

which allows for deducing $N_{\text{add}}$, given that the last term is known or insignificant. Figure S4 shows the same data as plotted in the lowest curve in Fig. 2e in main text, but now plotted as a function of $N_{\text{in}}$, instead of the noise source temperature, recovering the expected linear behavior. The linear fit provides the same result as the fits in Fig. 2e. Note that this method is independent of $F$, and that the effect of technical noise is negligible at large gain $G$, here satisfied approximately when $G \gtrsim 25$ dB.

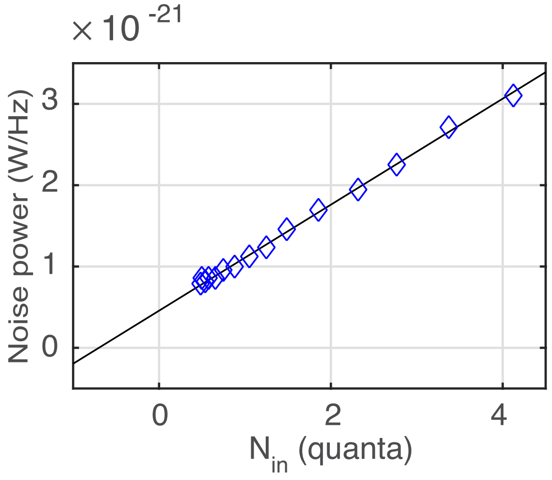


FIG. S4. *Noise calibration on linear scale.* Data from the lowest curve in Fig. 2e in the main text as a function of input noise quanta. The solid line is a linear fit.

Equation (S4) holds also for the phase-sensitive mode of operation. In addition to what discussed above, the measurement is repeated for all the desired quadrature angles. The data, complete with quantum noise fits similar to Fig. 2e in main text are shown in Fig. S5. From the fits we obtain the noise data in Fig. 3b in main text.

In Fig. S6 we show the measurement of the effective added noise $N_F$ of the entire microwave measurement system following the sample. This figure is likely dominated by the cryogenic amplifier because it has a high gain. This noise is measured the same way as the added noise of the optomechanical device, however, without any pump tones applied. This way, the sample acts as a slightly absorbing mirror. By changing the temperature of the noise calibration resistor,

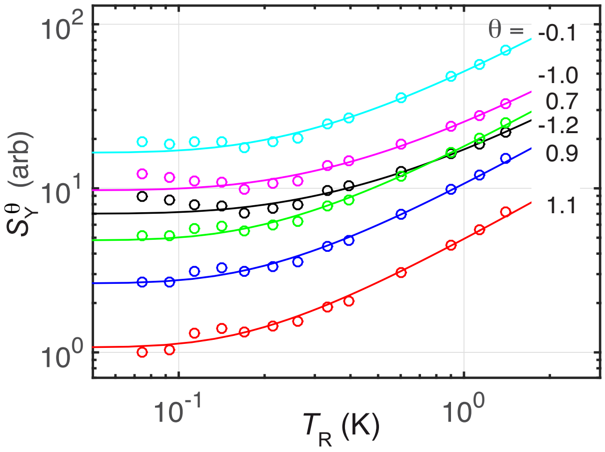


FIG. S5. *Phase-sensitive noise.* Noise calibration with the homodyne detection for Fig. 3b in main text, at different LO phases as indicated.

we observe a linearly increasing noise power when plotted as a function of the number of input noise quanta as seen in Fig. S6, obtaining $N_F \simeq 18 \pm 2$.

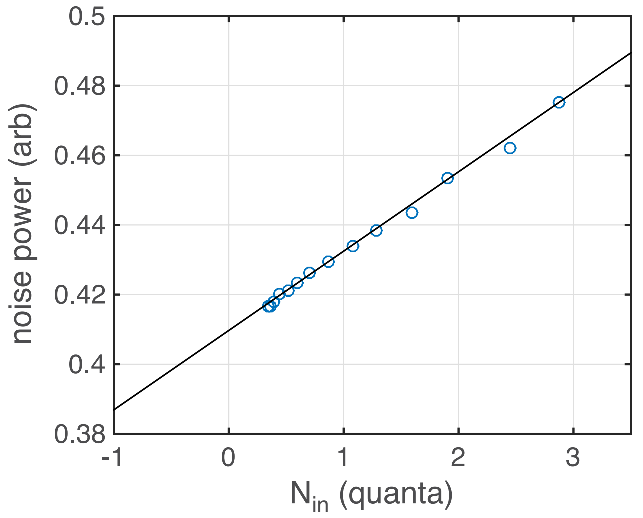


FIG. S6. *Noise of the cryogenic amplifier.* Noise at the output measured without any pump tones applied.

In Fig. S7 we show additional data similar to Fig. 2c and d in main text, but measured with a higher pump power. The gain profile is smoother because the two peaks start to overlap, but the noise is slightly worsened presumably because dielectric heating affects the mechanics bath temperature.

## C. Dynamic range of the amplification

A figure of merit for an amplifier is how large powers can be applied to the input before saturation takes place. This is important because in many applications (such as microwave optomechanics), strong coherent pump tones are present, and they can saturate the amplifier. The power handling capability is often characterized with the 1 dB compression point, which is the input power where the gain has dropped by 1 dB. Its value depends on the gain in the linear regime. We measured the gain as a function of the input power as seen in Fig. S8. When the gain is 22 dB for instance, 1 dB compression occurs at approximately -80 dBm.

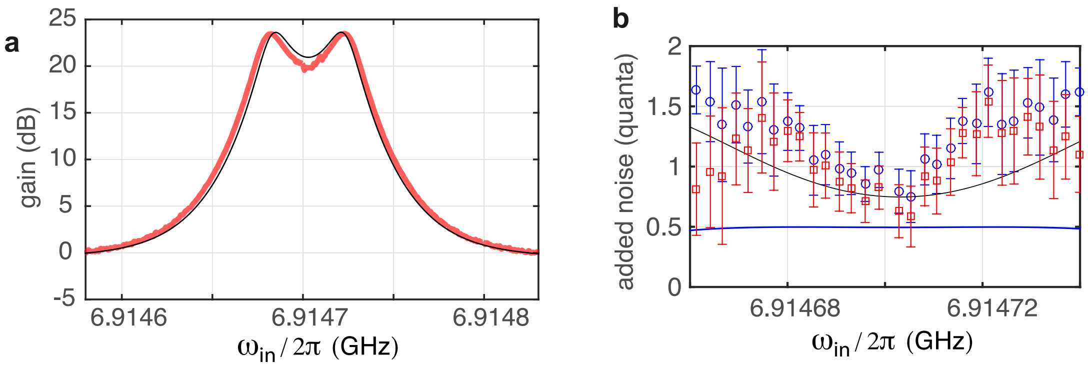


FIG. S7. *Gain and added noise.* Similar to Fig. 2c,d in main text, but higher pump power $G_-/2\pi \simeq 413$ kHz. **a**, Gain. **b**, The corresponding added noise.

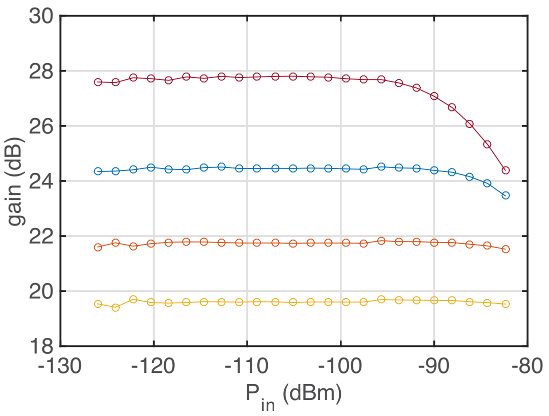


FIG. S8. *Power handling.* Gain as a function of input power at different input frequencies corresponding to different gains. Parameters are $G_-/2\pi \simeq 580$ kHz, $\delta/2\pi \simeq 900$ kHz.

### D. Calibration of squeezing

As in the main text, in the following the quantities written with a superscript $\theta$ refer to a specific quadrature, whereas those without the superscript are summed over the quadratures. We discuss the squeezing measured in the input of the hemt amplifier. The variables labeled with the letter $N$ are the spectral densities in units of quanta at the hemt input, and those at the output are labeled with $S$. The calibration of the amount of squeezing is done by using as a reference the noise level in one quadrature $S^\theta_{\rm off}$ when the pumps are off, equaling half the true input noise $N_{\rm hemt} = 2N^\theta_{\rm hemt}$ of the hemt. When the pumps are on or off, respectively, the measured noise is

$$S^\theta = G(N^\theta + N^\theta_{\rm hemt}) \tag{S6}$$

$$S^\theta_{\rm off} = G(N^\theta_{\rm off} + N^\theta_{\rm hemt}) \tag{S7}$$

Here, $N^\theta$ is the quantity of interest, the (possibly) squeezed noise radiating into the hemt input. $N^\theta_{\rm off} = N^\theta_{zp} + N^\theta_0$ can be larger than the vacuum value $N^\theta_{zp} = 1/4 = N_{zp}/2$ because of a possibly present extra thermal noise $N^\theta_0$.

The amount of squeezing is conveniently expressed as the noise in one quadrature in units of $N^\theta_{zp}$. The quantity plotted in Fig. 4 in the main text is

$$\text{squeezing} = \frac{N^\theta}{N^\theta_{zp}}\,, \tag{S8}$$

and hence a value $< 1$ (or 0 dB) entails squeezing below vacuum. Using Eqs. (S6,S7), Eq. (S8) becomes

$$\text{squeezing} = \frac{S^\theta/G - N^\theta_{\rm hemt}}{N^\theta_{zp}} \simeq \frac{N^\theta_{\rm hemt}\left(\frac{S^\theta}{S^\theta_{\rm off}} - 1\right)}{N^\theta_{zp}} \tag{S9}$$

A caveat in using Eq. (S9) is that in the present setting we cannot directly measure $N_{\rm hemt}$. What we can accurately measure is the effective input noise $N_F = N_{\rm hemt}/t$ , which includes the (power) transmission $t < 1$ between the sample and the hemt. In our system with a standard superconducting coaxial cabling, we estimate a typical $t \sim 1.5...2.5$ dB, which leads to relatively large error bars to the measured squeezing. We note that if for some reason the attenuation would be larger than we estimate, the squeezing would be stronger than claimed now. The attenuation is unlikely to be smaller than the stated values because even if all components are working ideally, the total attenuation amounts to approximately 1.5 dB.

At the high pump powers used in the squeezing demonstration, we observe that the noise calibration resistor heats up so that it stays at $\sim 160$ mK (Fig. S9a), hence emitting $N_0 \simeq 0.14$ quanta of extra thermal noise, as included in Eq. (S7). However, $N_0$ is compared to $N_{\rm hemt}$ and becomes negligible.

From the theory, we obtain the squeezing directly at the output of the sample. Losses between the sample and the hemt input, however, reduce the amount of squeezing by bringing the state towards a thermal state. In order to compare the data to theory, we make a rough estimation that the difference of the squeezing from vacuum is reduced by the attenuation $t$. The theoretical predictions in Fig. 4 in main text are obtained this way. In Fig. S9b we include also the predicted squeezing at the sample plane.

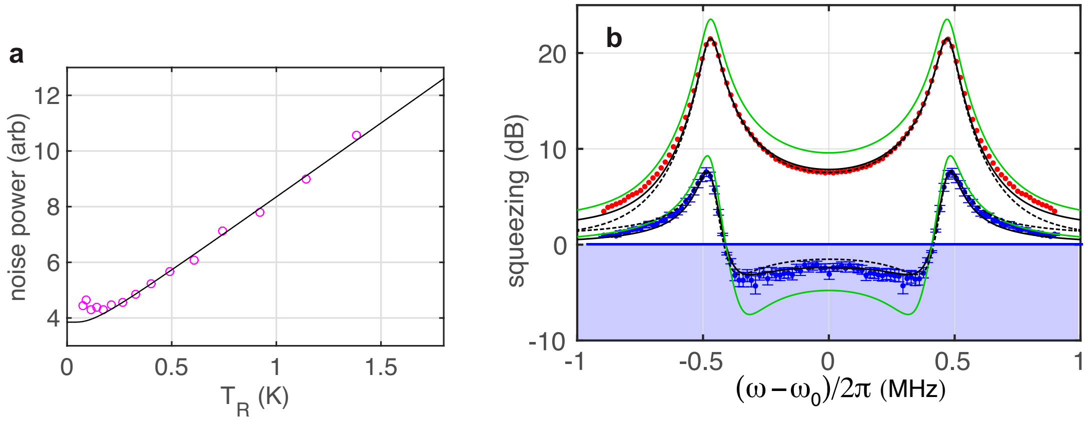


FIG. S9. *Squeezing analysis, $G_-/2\pi \simeq 690$ kHz, $G_+/2\pi \simeq 590$ kHz.* **a**, Thermal calibration with the heated resistor. **b**, Data of Fig. 4c in main text replotted, augmented with predicted squeezing without cavity parametric modulation (dashed black lines), and predicted squeezing at the sample output (green lines).

As in Ref. 19, in phase-sensitive measurements, we obtain the best fit by introducing a direct parametric modulation (amplitude $\sim (2\pi)\cdot 320$ kHz) of the cavity beyond the ideal optomechanical model. Although the parametric modulation somewhat enhances the squeezing and is needed to quantitatively understand the data, the observed squeezing is essentially of optomechanical origin. This can be seen in Fig. S9b, which also shows theory curves plotted without the cavity parametric term.

## II. THEORETICAL DETAILS

In this section we outline the theoretical model presented in detail in Ref. [8]. In section II B, we introduce a new interpretation of the operation of the phase-sensitive optomechanical amplifier.

### A. Equations of motion

The system Hamiltonian (Eq. (1) of the main text), expressed in terms of cavity Bogoliubov modes, can be derived from the conventional linearised optomechanical Hamiltonian,

$$\begin{aligned} H =& \omega_c a^\dagger a + \omega_c b^\dagger b \\ &+ \left(G_+ e^{-i\omega_+ t} + G_- e^{-i\omega_- t}\right)\left(a^\dagger b^\dagger + a^\dagger b\right) + \mathtt{h.c.} \end{aligned} \tag{S10}$$

Neglecting fast oscillating terms (rotating-wave approximation) and moving to a frame rotating at $\omega_c$ and $\omega_m - \delta$ for the cavity and the mechanical field respectively, we can write Eq. (S10) as

$$H = \delta\, b^\dagger b + G_+ a^\dagger b^\dagger + G_- a^\dagger b + \text{h.c.} \tag{S11}$$

Due to the symmetry induced by the linearisation scheme it is possible to recast Eq. (S11) in terms of Bogoliubov modes for either the mechanical field

$$H = \delta\left[\cosh^2\xi + \sinh^2\xi\right]\beta^\dagger\beta + \delta\cosh\xi\sinh\xi\left({\beta^\dagger}^2 + \beta^2\right) + G_{\rm BG}\left(a^\dagger\beta + a\beta^\dagger\right) \tag{S12}$$

or for the cavity field

$$H = \delta\, b^\dagger b + G_{\rm BG}\left(\alpha^\dagger b + \alpha b^\dagger\right), \tag{S13}$$

where $\beta = \cosh\xi\, b + \sinh\xi\, b^\dagger$ and $\alpha = \cosh\xi\, a + \sinh\xi\, a^\dagger$, $\cosh\xi = G_-/\sqrt{G_-^2 - G_+^2}$, $\sinh\xi = G_+/\sqrt{G_-^2 - G_+^2}$. With a view to the physics discussed in the main text, we focus on the form given by Eq. (S13), where the beam-splitter term $G_{\rm BG}\left(\alpha^\dagger b + \alpha b^\dagger\right)$ points towards the cooling of the mechanical motion to the temperature of the Bogoliubov cavity mode, and entails squeezing of the original cavity mode $a$.

From Eq. (S13) we can determine the following quantum Langevin equations in the frequency domain [1] for $\alpha$ and $b$

$$\begin{aligned} -i\omega\alpha_\omega &= -iG_{\rm BG}b_\omega - \frac{\kappa}{2}\alpha_\omega + \sqrt{\kappa}\alpha_{{\rm in}\,\omega} \\ -i\omega b_\omega &= -i\delta b_\omega + iG_{\rm BG}\alpha_\omega - \frac{\gamma}{2}b_\omega + \sqrt{\gamma}b_{{\rm in}\,\omega}. \end{aligned} \tag{S14}$$

The mechanical degrees of freedom can be eliminated from Eq. (S14), leading to the following equation for the Bogoliubov mode $\alpha$

$$-i\omega\alpha_\omega = G_{\rm BG}^2\chi_m\alpha_\omega - \frac{\kappa}{2}\alpha_\omega + \sqrt{\kappa}\alpha_{{\rm in}\,\omega} - iG_{\rm BG}\chi_m\sqrt{\gamma}b_{{\rm in}\,\omega}\,, \tag{S15}$$

where $\chi_m = [\gamma/2 - i\,(\omega-\delta)]^{-1}$.

Equation (S15) can be solved to give

$$\alpha_\omega = \chi_c^{\rm eff}\sqrt{\tilde\kappa}\tilde\alpha_{{\rm in}\,\omega} \tag{S16}$$

where

$$\begin{aligned} \chi_c^{\rm eff} &= \frac{1}{\kappa/2 - i\omega + G_{\rm BG}^2\chi_m} \\ \sqrt{\tilde\kappa}\tilde\alpha_{{\rm in}\,\omega} &= \sqrt{\kappa}\alpha_{{\rm in}\,\omega} - iG_{\rm BG}\chi_m\sqrt{\gamma}b_{{\rm in}\,\omega} \end{aligned} \tag{S17}$$

The output field $\alpha_{{\rm o}\,\omega}$ in terms of the input modes $\alpha_{{\rm in}\,\omega}$ is the obtained from

$$\alpha_{{\rm o}\,\omega} = \sqrt{\kappa}\alpha_\omega - \alpha_{{\rm in}\,\omega} \tag{S18}$$

The gains and added noise are then obtained as detailed e.g. in Ref. [12].

### B. Phase-sensitive amplification via phase-sensitively reflected Bogoliubov wave

As stated in the main text, Eq. (S13) represents the Hamiltonian of a beam splitter, and coincides with the Hamiltonian describing the cooling of a mechanical resonator by means of the coupling to a cavity Bogoliubov mode. Therefore, while it is natural to assume that the mechanics – albeit sub-optimally, due to the presence of $\delta$ – is cooled by the coupling with the Bogoliubov mode, the resulting phase-sensitive amplification for the output field is more surprising. The discussion of the system in terms of an ideal parametric amplifier can be understood in a somehow simplified picture in terms of phase shifts induced by the cavity coupled to the mechanical resonator. Since we focus here on the simplified analysis of the amplification process, we neglect all noise sources described above. We can write the I/O equations for the output field from Eq. (S13) as

$$\alpha_{{\rm o}\,\omega} = \left(\chi_c^{\rm eff} - 1\right)\sqrt{\kappa}\alpha_{{\rm in}\,\omega}\,. \tag{S19}$$

Since the cavity is overcoupled ($\kappa_{\rm e} \simeq \kappa$), we have that $\left|\chi_c^{\rm eff}(\omega) - 1\right| = \left|\chi_c^{\rm eff*}(-\omega) - 1\right| \simeq 1$. Defining the phases of the reflected cavity modes at frequencies $\pm\omega$, $\phi_\omega^+ \equiv {\rm Arg}\left[\chi_c^{\rm eff}(\omega) - 1\right]$ and $\phi_\omega^- \equiv {\rm Arg}\left[\chi_c^{\rm eff*}(-\omega) - 1\right]$, we can write the I/O equation for the original output modes $a_{{\rm o}\,\omega}$ as

$$\begin{aligned} a_{{\rm o}\,\omega} &= \cosh\xi\alpha_{{\rm o}\,\omega} - \sinh\xi\alpha_{{\rm o}\,-\omega}^\dagger \\ &= \left|\chi_c^{\rm eff}(\omega) - 1\right|\left(\cosh\xi e^{i\phi_\omega^+}\alpha_{{\rm in}\,\omega} - \sinh\xi e^{i\phi_\omega^-}\alpha_{{\rm in}\,-\omega}^\dagger\right) \\ &= \left(\cosh^2\xi e^{i\phi_\omega^+} - \sinh^2\xi e^{i\phi_\omega^-}\right)a_{{\rm in}\,\omega} - \cosh\xi\sinh\xi\left(e^{i\phi_\omega^+} - e^{i\phi_\omega^-}\right)a_{{\rm in}\,-\omega}^\dagger. \end{aligned} \tag{S20}$$

For $\delta \geq 4G_{BG}^2/\kappa$, to the first order in $G_{\rm BG}/\kappa$ and $\delta/\kappa$, we have

$$\begin{aligned} \phi_{-\omega_{\rm max}}^+ &= \pi + \frac{2}{\kappa}\left(\frac{2G_{\rm BG}^2}{\delta} - 2\delta\right) \\ \phi_{-\omega_{\rm max}}^- &= -4\frac{\delta}{\kappa} \end{aligned} \tag{S21}$$

and

$$\begin{aligned}\phi^{+}_{\omega_{\max}} =& 4\frac{\delta}{\kappa}\\ \phi^{-}_{\omega_{\max}} =& \pi - \frac{2}{\kappa}\left(\frac{2G_{\mathrm{BG}}^2}{\delta} - 2\delta\right)\end{aligned} \tag{S22}$$

Focusing on $\omega = \omega_{\max}$, and neglecting the small $1/\kappa$ terms, Eq. (S20) can be written as

$$a_{\mathrm{o}\,\omega} = \left(\cosh^2\xi + \sinh\xi^2\right) a_{\mathrm{in}\,\omega} - 2\cosh\xi\sinh\xi a^{\dagger}_{\mathrm{in}\,-\omega}. \tag{S23}$$

It is possible to recognize in this expression the relation for a phase-sensitive amplifier. In this case the gains in the preferred quadratures are given by

$$\begin{aligned}\mathcal{G}_1 = (\cosh\xi + \sinh\xi)^2 = \frac{G_+ + G_-}{G_+ - G_-} = \exp(2\xi)\\ \mathcal{G}_2 = (\cosh\xi - \sinh\xi)^2 = \frac{G_+ - G_-}{G_+ + G_-} = \exp(-2\xi)\,.\end{aligned} \tag{S24}$$

Thus the amplifier in this limit behaves like an ideal parametric amplifier. We note also that the expression for the square of the gain $\mathcal{G}_1^2$ can be recast as

$$\mathcal{G}_1^2 = \left(1 + \frac{2G_+G_-}{G_+^2 - G_-^2}\right)^2 \overset{G_+ \to G_-}{=} \frac{4G_+^2G_-^2}{\left(G_+^2 - G_-^2\right)^2}\,, \tag{S25}$$

On the other hand, for $\delta \simeq 0$, $\phi^{+}_{\omega_{\max}} = \phi^{-}_{\omega_{\max}} = \phi^{+}_{-\omega_{\max}} = \phi^{-}_{-\omega_{\max}} = 0$, and Eq. (S20) leads to the (trivial) I/O relation

$$a_{\mathrm{o}\,\omega} = a_{\mathrm{in}\,\omega}\,, \tag{S26}$$

describing the complete reflection without any amplification.

---

[1] The subscript $\omega$ stands for the frequency, and we use the Fourier convention where $a^{\dagger}_{\omega}$ is the conjugate of $a_{\omega}$.
